# Supplementary material for: Integrating Variable Reduction Strategy with Evolutionary Algorithm for Solving Nonlinear Equations Systems
Source: arXiv:2008.04223 source file (2020-07-13)
Supplement: Supplementary file 1 [file supplement_file_of_VRS_with_EA_for_NESs.pdf]

# Supplemental material for "Integrating Variable Reduction Strategy with Evolutionary Algorithm for Solving Nonlinear Equations Systems"

The specific expressions, decision space, the actual known roots and the selected reduction schemes for F01-E46 are as follows:

(1) E1:

$$\begin{cases} x_1^2 - x_2^2 = 0 & (1) \\ 1 - |x_1 - x_2| = 0 & (2) \end{cases} \tag{1}$$

where $x_i \in [-3,3]$, $i = 1,2$. It has two roots: (-0.5,0.5) and (0.5,-0.5).

The equation (1) is the eliminated equation. $x_1$ is the reduced variable. We can get the following variable reduction scheme:

$$x_1 = \pm x_2 \tag{2}$$

(2) E2:

$$\begin{cases} x_1^2 - x_2 - 2 = 0 & (1) \\ x_1 + \sin(\frac{\pi x_2}{2}) = 0 & (2) \end{cases} \tag{3}$$

where $x_i \in [-3,3]$, $i = 1,2$. It has three roots: (1,-1), (0,-2) and (0.7075,-1.5).

The equation (2) is the eliminated equation. $x_1$ is the reduced variable. We can get the following variable reduction scheme:

$$x_1 = -\sin(\frac{\pi x_2}{2}) \tag{4}$$

(3) E3:

$$\begin{cases} x_1 x_2 + (x_1 - 2x_3)(x_2 - 2x_3) - 165 = 0 & (1) \\ \frac{x_1 x_2^3}{12} - \frac{(x_1 - 2x_3)(x_2 - 2x_3)^3}{12} - 9369 = 0 & (2) \\ \frac{2(x_2 - x_3)^2 (x_1 - x_3)^2 x_3}{x_1 + x_2 - 2x_3} - 6835 = 0 & (3) \end{cases} \tag{5}$$

where $x_i \in [0,50]$, $i = 1,2,3$. It has two roots: (43.155566,10.128950,12.944048) and (7.602995,24.541982,11.576716).

The equation (2) is the eliminated equation. $x_1$ is the reduced variable. We can get the following variable reduction scheme:

$$x_1 = \frac{(x_3 (x_2 - 2x_3)^3)/6 - 9369}{(x_2 - 2x_3)^3 - x_2^3/12} \tag{6}$$

(4) E4:

$$\begin{cases} x_1 + x_2 - 3 = 0 & (1) \\ x_1^2 + x_2^2 - 9 = 0 & (2) \end{cases} \tag{7}$$

where $x_i \in [-3,3]$, $i = 1,2$. It has two roots: (0,3) and (3,0).

The equation (1) is the eliminated equation. $x_1$ is the reduced variable. We can get the following variable reduction scheme:

$$x_1 = 3 - x_2 \tag{8}$$

(5) E5:

$$\begin{cases} x_1 - \sin(2x_1 + 3x_2) - \cos(3x_1 - 5x_2) = 0 & (1) \\ x_2 - \sin(x_1 - 2x_2) + \cos(x_1 + 3x_2) = 0 & (2) \end{cases} \tag{9}$$

where $x_i \in [-3,3]$, $i = 1,2$. It has three roots: (-0.173346,-0.256091), (0.838835,0.537119) and (0.792693,0.138017).

(6) E6:

$$\begin{cases} e^{x_1^2} - 8x_1 \sin(x_2) = 0 & (1) \\ x_1 + x_2 - 1 = 0 & (2) \\ (x_3 - 1)^3 = 0 & (3) \end{cases} \tag{10}$$

where $x_i \in [0,1]$, $i = 1,2,3$. It has two roots: (0.673584,0.326416,1) and (0,1,1).

The equation (2) and (3) are the eliminated equations. $x_2$ and $x_3$ are the reduced variables. We can get the following variable reduction scheme:

$$\begin{aligned} x_2 &= 1 - x_1 \\ x_3 &= 1 \end{aligned} \tag{11}$$

(7) E7:

$$\begin{cases} x_1^3 - 3x_1 x_2^2 - 1 = 0 & (1) \\ 3x_1^2 x_2 - x_2^3 + 1 = 0 & (2) \end{cases} \tag{12}$$

where $x_i \in [-1,2]$, $i = 1,2$. It has three roots: (-0.290515,1.084215), (1.084215,-0.290515) and (-0.793701,-0.793701).

The equation (1) is the eliminated equation. $x_2$ is the reduced variable. We can get the following variable reduction scheme:

$$x_2 = \pm\sqrt{\frac{x_1^3 - 1}{3x_1}} \tag{13}$$

(8) E8:

$$\begin{cases} x_1^2 + x_2^2 - 1 = 0 & (1) \\ x_1 - x_2 = 0 & (2) \end{cases} \tag{14}$$

where $x_i \in [-1,1]$, $i = 1,2$. It has two roots: $(-0.707107, -0.707107)$ and $(0.707107, 0.707107)$.

The equation (2) is the eliminated equation. $x_1$ is the reduced variable. We can get the following variable reduction scheme:

$$x_2 = x_1 \tag{15}$$

(9) E9:

$$\begin{cases} \sum_{i=1}^{D} x_i^2 - 1 = 0 & (1) \\ | x_1 - x_2 | + \sum_{i=3}^{D} x_i^2 = 0 & (2) \end{cases} \tag{16}$$

where $x_i \in [-1,1]$, $i = 1,2,\ldots,20$. It has two roots: $(-0.707107, -0.707107, 0, \cdots, 0)$ and $(0.707107, 0.707107, 0, \cdots, 0)$.

The equation (1) is the eliminated equation. $x_2$ is the reduced variable. We can get the following variable reduction scheme:

$$x_2 = \pm\sqrt{1 - (x_1^2 + \sum_{i=3}^{D} x_i^2)} \tag{17}$$

(10) E10:

$$\begin{cases} x_1 - \sin(5\pi x_2) = 0 & (1) \\ x_1 - x_2 = 0 & (2) \end{cases} \tag{18}$$

where $x_i \in [-1,1]$, $i = 1,2$. It has 11 roots: (-0.924840, -0.924840), (-0.866760, -0.866760), (-0.562010, -0.562010), (-0.428168, -0.428168), (-0.187960, -0.187960), (0.000000, 0.000000), (0.924840, 0.924840), (0.866760, 0.866760), (0.562010, 0.562010), (0.428168, 0.428168) and (0.187960, 0.187960).

The equation (2) is the eliminated equation. $x_2$ is the reduced variable. We can get the following variable reduction scheme:

$$x_2 = x_1 \tag{19}$$

(11) E11:

$$\begin{cases} x_1 - \cos(4\pi x_2) = 0 & (1) \\ x_1^2 + x_2^2 = 1 & (2) \end{cases} \tag{20}$$

where $x_i \in [-1,1]$, $i = 1,2$. It has 15 roots: (0.416408, -0.909178), (-0.561364, -0.827569), (-0.724322, -0.689463), (0.837812, -0.545959), (0.886984, -0.461799), (-0.962322, -0.271914), (-0.972855, -0.231415), (1.000000, 0.000000) , (0.416408, 0.909178), (-0.561364, 0.827569), (-0.724322, 0.689463), (0.837812, 0.545959), (0.886984, 0.461799), (-0.962322, 0.271914) and (-0.972855, 0.231415).

The equation (1) is the eliminated equation. $x_1$ is the reduced variable. We can get the following variable reduction scheme:

$$x_1 = \cos(4\pi x_2) \tag{21}$$

(12) E12:

$$\begin{cases} \cos(2x_1) - \cos(2x_2) - 0.4 = 0 & (1) \\ 2(x_2 - x_1) + \sin(2x_2) - \sin(2x_1) - 1.2 = 0 & (2) \end{cases} \tag{22}$$

where $x_i \in [-10,10]$, $i = 1,2$. It has 13 roots: (-9.268258, -8.931402), (-8.744542, -7.164787), (-6.126665, -5.789809), (-5.602950, -4.023195), (-2.985073, -2.648216), (-2.461357, -0.881602), (-0.156520, 0.493376), (0.680236, 2.259991), (3.298113, 3.634969), (3.821828, 5.401583), (6.439705, 6.776562), (6.963421, 8.543176) and (9.581298,9.918154).

(13) E13- Interval arithmetic benchmark:

$$\begin{cases} x_1 - 0.25428722 - 0.18324757 x_4 x_3 x_9 = 0 & (1) \\ x_2 - 0.37842197 - 0.16275449 x_1 x_{10} x_6 = 0 & (2) \\ x_3 - 0.27162577 - 0.16955071 x_1 x_2 x_{10} = 0 & (3) \\ x_4 - 0.19807914 - 0.15585316 x_7 x_1 x_6 = 0 & (4) \\ x_5 - 0.44166728 - 0.19950920 x_7 x_6 x_3 = 0 & (5) \\ x_6 - 0.14654113 - 0.18922793 x_8 x_5 x_{10} = 0 & (6) \\ x_7 - 0.42937161 - 0.21180486 x_2 x_5 x_8 = 0 & (7) \\ x_8 - 0.07056438 - 0.17081208 x_1 x_7 x_6 = 0 & (8) \\ x_9 - 0.34504906 - 0.19615740 x_{10} x_6 x_8 = 0 & (9) \\ x_{10} - 0.42651102 - 0.21466544 x_4 x_8 x_1 = 0 & (10) \end{cases} \tag{23}$$

where $x_i \in [-2,2]$, $i = 1,2,\cdots,10$. It has one root: (0.257833, 0.381097, 0.278745, 0.200669, 0.445251, 0.149184, 0.432010, 0.073403, 0.345967, 0.427326).

The equation (1), (6), (7) and (10) are the eliminated equations. $x_1$, $x_6$, $x_7$ and $x_{10}$ are the reduced variables. We can get the following variable reduction scheme:

$$\begin{aligned} x_1 &= 0.18324757x_3x_9x_6 + 0.25428722 \\ x_6 &= 0.00744364x_3x_5x_9x_4^2x_8^2 + 0.01032932x_5x_4x_8^2 + 0.08070780x_5x_8 + 0.14654113 \\ x_7 &= 0.21180486x_2x_5x_8 + 0.42937161 \\ x_{10} &= 0.03933692x_3x_8x_9x_4^2 + 0.05458668x_8x_4 + 0.42651102 \end{aligned} \quad (24)$$

(14) E14:

$$\begin{cases} 100(x_1 - 0.25) = 0 & (1) \\ 100(x_1 \sin(4\pi x_2^2) + 0.75x_1 - 0.25) = 0 & (2) \end{cases} \quad (25)$$

where $x_i \in [-1,1]$, $i = 1,2$. It has 8 roots: (0.250000, -0.854337), (0.250000, -0.721185), (0.250000, -0.479471), (0.250000, -0.141801), (0.250000, 0.141801), (0.250000, 0.479471), (0.250000, 0.721185) and (0.250000, 0.854337).

The equation (1) is the eliminated equation. $x_1$ is the reduced variable. We can get the following variable reduction scheme:

$$x_1 = 0.25 \quad (26)$$

(15) E15:

$$\begin{cases} 3 - x_1x_3^2 = 0 & (1) \\ x_3\sin(\frac{\pi}{x_2}) - x_3 - x_4 = 0 & (2) \\ -x_2x_3e^{(1-x_1x_3)} + 0.2707 = 0 & (3) \\ 2x_1^2x_3 - x_2^4x_3 - x_2 = 0 & (4) \end{cases} \quad (27)$$

where $x_i \in [0,5]$, $i = 1,2,\cdots,4$. It has one root: (3, 2, 1, 0).

The equation (1), (2) and (3) are the eliminated equations. $x_2$ $x_3$ and $x_4$ are the reduced variables. We can get the following variable reduction scheme:

$$\begin{aligned} x_2 &= \frac{0.2707}{\sqrt{\frac{3}{x_1}}e^{(1-x_1\sqrt{\frac{3}{x_1}})}} \\ x_3 &= \sqrt{\frac{3}{x_1}} \\ x_4 &= \sqrt{\frac{3}{x_1}}\sin(\frac{\pi\sqrt{\frac{3}{x_1}}e^{(1-x_1\sqrt{\frac{3}{x_1}})}}{0.2707} - \sqrt{\frac{3}{x_1}}) \end{aligned} \quad (28)$$

(16) E16:

$$\begin{cases} (1-\mathrm{R})(\frac{\mathrm{H}}{10(1+\beta_1)} - x_1)e^{(\frac{10x_1}{1+\frac{10x_1}{\gamma}})} - x_1 = 0 & (1) \\ (1-\mathrm{R})(\frac{\mathrm{H}}{10} - \beta_1x_1 - (1+\beta_2)x_2)e^{(\frac{10x_2}{1+\frac{10x_2}{\gamma}})} + x_1 - (1+\beta_2)x_2 = 0 & (2) \end{cases} \quad (29)$$

where $x_i \in [0,1]$, $i = 1,2$, $\mathrm{R} = 0.96$, $\mathrm{H} = 11$, $\gamma = 1000$, $\beta_1 = \beta_2 = 2$. It has 7 roots: (0.042100, 0.061813), (0.042100, 0.268723), (0.266600, 0.178430), (0.266600, 0.327267), (0.266600, 0.461111), (0.042318, 0.686779) and (0.719074, 0.244164).

The equation (2) is the eliminated equation. $x_1$ is the reduced variable. We can get the following variable reduction scheme:

$$x_1 = -(3x_2 + \frac{1}{25}\mathrm{e}^{\frac{10x_2}{1+\frac{x_2}{100}}}(3x_2 - \frac{11}{5}))/(\frac{2}{25}\mathrm{e}^{\frac{10x_2}{1+\frac{x_2}{100}}} - 1) \quad (30)$$

(17) E17:

$$\begin{cases} 2x_1 + x_2 + x_3 + x_4 + x_5 - 6.0 = 0 & (1) \\ x_1 + 2x_2 + x_3 + x_4 + x_5 - 6.0 = 0 & (2) \\ x_1 + x_2 + 2x_3 + x_4 + x_5 - 6.0 = 0 & (3) \\ x_1 + x_2 + x_3 + 2x_4 + x_5 - 6.0 = 0 & (4) \\ x_1x_2x_3x_4x_5 - 1.0 = 0 & (5) \end{cases} \quad (31)$$

where $x_i \in [-10,10]$, $i = 1,2,\cdots,5$. It has three roots: (1,1,1,1,1), (0.916355,0.916355,0.916355,0.916355,1.418227) and (-0.579043, -0.579043, -0.579043, -0.579043,8.895215).

The equation (1), (2), (3) and (4) are the eliminated equations. $x_1$, $x_2$, $x_3$ and $x_4$ are the reduced variables. We can get the following variable reduction scheme:

$$x_1 = x_2 = x_3 = x_4 = \frac{6 - x_5}{5} \quad (32)$$

(18) E18:

$$\begin{cases} x_1 + x_2^4 x_4 x_6 / 2 + 0.75 = 0 & (1) \\ x_2 + 0.405 e^{1+x_1 x_2} - 1.405 = 0 & (2) \\ x_3 - x_4 x_6 / 2 + 1.5 = 0 & (3) \\ x_4 - 0.605 e^{1-x_3^2} = 0.395 = 0 & (4) \\ x_5 - x_2 x_6 / 2 + 1.5 = 0 & (5) \\ x_6 - x_1 x_5 = 0 & (6) \end{cases} \quad (33)$$

where $x_i \in [-1,1]$, $i = 1,2,\cdots,6$. It has one root: $(-1,1,1,1,-1,1)$.

The equation (1) (3), (5) and (6) are the eliminated equations. $x_1$, $x_4$, $x_5$ and $x_6$ are the reduced variables. We can get the following variable reduction scheme:

$$\begin{aligned} x_1 &= -0.5x_1^4 x_2 - 0.75x_1^4 - 0.75 \\ x_4 &= \frac{1}{3}\frac{(2x_2+3)(3.0x_1 + 2x_1^5 x_2 + 3x_1^5 + 8)}{(2x_1^4 x_2 + 3x_1^4 + 3)} \\ x_5 &= \frac{-12}{(3x_1 + 2x_1^5 x_2 + 3x_1^5 + 8)} \\ x_6 &= \frac{3(2x_1^4 x_2 + 3x_1^4 + 3)}{(3x_1 + 2x_1^5 x_2 + 3x_1^5 + 8)} \end{aligned} \quad (34)$$

(19) E19:

$$\begin{cases} \sin(x_1^3) - 3x_1 x_2^2 - 1 = 0 & (1) \\ \cos(3x_1^2 x_2) - |x_2^3| + 1 = 0 & (2) \end{cases} \quad (35)$$

where $x_i \in [-2,2]$, $i = 1,2$. It has 10 roots: (-1.810885, -0.349092), (-1.810885, 0.349092), (-1.502221, -0.409077), (-1.502221, 0.409077), (-1.791302, 0.301926), (-1.791302, -0.301926), (-0.947268, 0.785020), (-0.947268, -0.785020), (-0.213057, 1.256845) and (-0.213057, -1.256845).

The equation (1) is the eliminated equation. $x_2$ is the reduced variable. We can get the following variable reduction scheme:

$$x_2 = \pm\sqrt{\frac{\sin(x_1^3) - 1}{3x_1}} \quad (36)$$

(20) E20:

$$\begin{cases} 4x_1^3 + 4x_1 x_2 + 2x_2^2 - 42x_1 - 14 = 0 & (1) \\ 4x_2^3 + 2x_1^2 + 4x_1 x_2 - 26x_2 - 22 = 0 & (2) \end{cases} \quad (37)$$

where $x_i \in [-5,5]$, $i = 1,2$. It has 9 roots: (-0.127961, -1.953715), (-0.270845, 2.884255), (0.086678, 0.073852), (3.385154, -1.848127), (3.584428, -1.848127), (3.000000, 2.000000), (-3.779310, -3.283186), (-3.073026, -0.081353) and (-2.805118,3.131313).

The equation (1) is the eliminated equation. $x_2$ is the reduced variable. We can get the following variable reduction scheme:

$$x_2 = -x_1 \pm \sqrt{-2x_1^3 + x_1^2 + 21x_1 + 7} \quad (38)$$

(21) E21:

$$\begin{cases} -\sin(x_1)\cos(x_2) - 2\cos(x_1)\sin(x_2) = 0 & (1) \\ -\cos(x_1)\sin(x_2) - 2\sin(x_1)\cos(x_2) = 0 & (2) \end{cases} \quad (39)$$

where $x_i \in [0, 2\pi]$, $i = 1,2$. It has 13 roots: (0.000000, 0.000000), (3.141593, 0.000000), (1.570796, 1.570796), (6.283185, 0.000000), (0.000000, 3.141593), (4.712389, 1.570796), (3.141593, 3.141593), (1.570796, 4.712389), (6.283185, 3.141593), (0.000000, 6.283185), (4.712389, 4.712389), (3.141593, 6.283185) and (6.283185, 6.283185)

(22) E22:

$$\begin{cases} x_1^2 + x_2^2 - 1.0 = 0 & (1) \\ x_3^2 + x_4^2 - 1.0 = 0 & (2) \\ x_5^2 + x_6^2 - 1.0 = 0 & (3) \\ x_7^2 + x_8^2 - 1.0 = 0 & (4) \\ 4.731\times10^{-3} x_1 x_3 - 0.3578 x_2 x_3 - 0.1238 x_1 + x_7 & \\ -1.637\times10^{-3} x_2 - 0.9338 x_4 - 0.3571 = 0 & (5) \\ 0.2238 x_1 x_3 + 0.7623 x_2 x_3 + 0.2638 x_1 - x_7 & \\ -0.07745 x_2 - 0.6734 x_4 - 0.6022 = 0 & (6) \\ x_6 x_8 + 0.3578 x_1 + 4.731\times10^{-3} x_2 = 0 & (7) \\ -0.7623 x_1 + 0.2238 x_2 + 0.3461 = 0 & (8) \end{cases} \quad (40)$$

where $x_i \in [-1,1]$, $i = 1,2,\cdots,8$. It has 16 roots as shown in Table S-1:

**Table S-1** The roots of E22

| $x_1$ | $x_2$ | $x_3$ | $x_4$ | $x_5$ | $x_6$ | $x_7$ | $x_8$ |
|---|---|---|---|---|---|---|---|
| 0.1644 | -0.9864 | -0.9471 | -0.3210 | -0.9982 | -0.0594 | 0.4110 | 0.9116 |
| 0.1644 | -0.9864 | -0.9471 | -0.3210 | -0.9982 | 0.0594 | 0.4110 | -0.9116 |

| | | | | | | | |
|---|---|---|---|---|---|---|---|
| 0.1644 | -0.9864 | -0.9471 | -0.3210 | 0.9982 | -0.0594 | 0.4110 | 0.9116 |
| 0.1644 | -0.9864 | -0.9471 | -0.3210 | 0.9982 | 0.0594 | 0.4110 | -0.9116 |
| 0.1644 | -0.9864 | 0.7185 | -0.9656 | -0.9980 | -0.0638 | -0.5278 | 0.8494 |
| 0.1644 | -0.9864 | 0.7185 | -0.9656 | -0.9980 | 0.0638 | -0.5278 | -0.8494 |
| 0.1644 | -0.9864 | 0.7185 | -0.9656 | 0.9980 | -0.0638 | -0.5278 | 0.8494 |
| 0.1644 | -0.9864 | 0.7185 | -0.9656 | 0.9980 | 0.0638 | -0.5278 | -0.8494 |
| 0.6716 | 0.7410 | -0.6516 | -0.7586 | -0.9625 | -0.2711 | -0.4376 | 0.8992 |
| 0.6716 | 0.7410 | -0.6516 | -0.7586 | -0.9625 | 0.2711 | -0.4376 | -0.8992 |
| 0.6716 | 0.7410 | -0.6516 | -0.7586 | 0.9625 | -0.2711 | -0.4376 | 0.8992 |
| 0.6716 | 0.7410 | -0.6516 | -0.7586 | 0.9625 | 0.2711 | -0.4376 | -0.8992 |
| 0.6716 | 0.7410 | 0.9519 | -0.3064 | -0.9638 | -0.2666 | 0.4046 | 0.9145 |
| 0.6716 | 0.7410 | 0.9519 | -0.3064 | -0.9638 | 0.2666 | 0.4046 | -0.9145 |
| 0.6716 | 0.7410 | 0.9519 | -0.3064 | 0.9638 | 0.2666 | 0.4046 | -0.9145 |
| 0.6716 | 0.7410 | 0.9519 | -0.3064 | 0.9638 | -0.2666 | 0.4046 | 0.9145 |

The equation (5), (6), (7) and (8) are the eliminated equations. $x_1$, $x_4$, $x_6$ and $x_7$ are the reduced variables. We can get the following variable reduction scheme:

$$\begin{aligned} &x_1=0.29358520x_2+0.45402073 \\ &x_4=0.06455304x_3-0.02363432x_2+0.29342213x_2x_3-0.55732771 \\ &x_6=-\frac{0.01311819(8.36820813x_2+12.383458)}{x_8} \\ &x_7=0.01591312x_2+0.05813982x_3+0.63041391x_2x_3-0.10712485 \end{aligned} \tag{41}$$

(23) E23:

$$\begin{cases} 4x_1^3-3x_1-\cos(x_2)=0 \quad (1) \\ \sin(x_1^2)-|x_2|=0 \quad (2) \end{cases} \tag{42}$$

where $x_i \in [-2,2]$, $i=1,2$. It has 6 roots: (-0.597167, -0.349098), (-0.597167, 0.349098), (-0.442798, -0.194781), (-0.442798, 0. 194781), (0.964499, -0.801774) and (0.964499, 0.801774).

The equation (1) is the eliminated equation. $x_2$ is the reduced variable. We can get the following variable reduction scheme:

$$x_2=\pm\sin(x_1^2) \tag{43}$$

(24) E24:

$$\begin{cases} x_i+\sum_{j=1}^{D}x_j-(D+1)=0,\ i=1,\cdots,D-1 \quad (1) \\ \prod_{j=1}^{D}x_j-1=0 \quad (2) \end{cases} \tag{44}$$

where $x_i \in [-2,2]$, $i=1,2,\cdots,20$ and $D=20$. It has two roots: $(-1,\cdots,1)$ and $(0.994922,\cdots,0.994922,1.101551)$.

The equations in the equation (1) are the eliminated equations. $x_k$, $k=1,2,\cdots,D-1$ are the reduced variable. We can get the following variable reduction scheme:

$$x_k=\frac{21-x_{20}}{20},\ k=1,2,\cdots,D-1 \tag{45}$$

(25) E25:

$$x_i-\cos(2x_i-\sum_{j=1}^{D}x_j)=0,\ i=1,\cdots,D \tag{46}$$

where $x_i \in [-1,1]$, $i=1,2,\cdots,D$ and $D=3$. It has 6 roots: (0.810561,0.810561, 0.625687), (0.810561, -0.625687, 0.810561), (-0.625687, 0.810561, 0.810561), (0.543850, 0.995778, 0.543850), (0.543850, 0.543850, 0.995778), (0.995778, 0.543850, 0.543850) and (0.739086, 0.739086, 0.739086).

The equation when $i=1$ in Eq. (46) is the eliminated equation. $x_3$ is the reduced variable. We can get the following variable reduction scheme:

$$x_3=x_1-x_2\pm\text{acos}(x_1) \tag{47}$$

(26) E26:

$$\begin{cases} x_1^2+x_2^2-2=0 \quad (1) \\ x_1^2+\frac{x_2^2}{4}-1=0 \quad (2) \end{cases} \tag{48}$$

where $x_i \in [-2,2]$, $i=1,2$, $D=3$. It has four roots: (-0.816497, -1.154701), (0.816497, -1.154701), (-0.816497, 1.154701) and (0.816497, 1.154701).

The equation (1) is the eliminated equation. $x_2$ is the reduced variable. We can get the following variable reduction scheme:

$$x_2=\pm\sqrt{2-x_1^2} \tag{49}$$

(27) E27:

$$\begin{cases} e^{x_1^2+x_2^2}-3=0 \quad (1) \\ |x_2|+x_1-\sin(3(|x_2|+x_1)) \quad (2) \end{cases} \tag{50}$$

where $x_i \in [-2,2]$, $i=1,2$. It has 6 roots: (-0.741152, -0.741152), (-0.741152, 0.741152), (-0.256625, 1.016246), (-0.256625, -1.016246), (-1.016246, -0.256625) and (-1.016246, 0.256625).

The equation (1) is the eliminated equation. $x_2$ is the reduced variable. We can get the following variable reduction scheme:

$$x_2 = \pm\sqrt{\ln 3 - x_1^2} \tag{51}$$

(28) E28:

$$\begin{cases} -3.84x_1^2 + 3.84x_1 - x_2 = 0\ (1) \\ -3.84x_2^2 + 3.84x_2 - x_3 = 0(2) \\ -3.84x_3^2 + 3.84x_3 - x_1 = 0\ (3) \end{cases} \tag{52}$$

where $x_i \in [0,1],\ i = 1,2,3$. It has 6 roots: (0.000000, 0.000000, 0.000000), (0.488122, 0.959435, 0.149452), (0.540304, 0.953754, 0.169399), (0.959447, 0.149373, 0.487917), (0.149440, 0.488092, 0.959440), (0.953781, 0.169343, 0.540157), (0.169254, 0.539937, 0.953788) and (0.739584, 0.739584, 0.739574)

The equation (1) and (2) is the eliminated equations. $x_2$ and $x_3$ are the reduced variables. We can get the following variable reduction scheme:

$$x_2 = \frac{96x_1 - 96x_1^2}{25}$$
$$x_3 = -\frac{884736x_1^4 + 1769472x_1^3 - 1115136x_1^2}{15625} + \frac{9216x_1}{625} \tag{53}$$

(29) E29:

$$\begin{cases} 3x_1^2 + \sin(x_1x_2) - x_3^2 + 2.0 = 0 \quad (1) \\ 2x_1^3 + x_2^2 - x_3 + 3.0 = 0 \quad (2) \\ \sin(2x_1) + \cos(x_2x_3) + x_2 - 1.0 = 0(3) \end{cases} \tag{54}$$

where $x_1 \in [-5,5],\ x_2 \in [-1,3],\ x_3 \in [-5,5]$. It has two roots: (-0.064417, 2.090440, -1.370473) and (-0.032759, 1.264629, 1.400644).

The equation (1) is regarded as the eliminated equation, and $x_3$ is the reduced variable. We can get the following variable reduction scheme:

$$x_3 = \pm\sqrt{3x_1^2 + \sin(x_1x_2) + 2.0} \tag{55}$$

(30) E30:

$$\begin{cases} 5x_1^9 - 6x_1^5x_2^2 + x_1x_2^4 + 2x_1x_3 = 0\ (1) \\ -2x_1^6x_2 + 2x_1^2x_2^3 + 2x_2x_3 = 0\ \ (2) \\ x_1^2 + x_2^2 - 0.265625 = 0 \quad (3) \end{cases} \tag{56}$$

where $x_1 \in [-0.6,0.6],\ x_2 \in [-0.6,0.6],\ x_3 \in [-2,5]$. It has 12 roots: (0.279855, 0.432789, -0.014189), (0.279855, -0.432789, -0.014189), (-0.279855, 0.432789, -0.014189), (-0.279855, -0.432789, -0.014189), (0.466980, 0.218070, 0.000000), (-0.466980, 0.218070, 0.000000), (0.466980, -0.218070, 0.000000), (-0.466980, -0.218070, 0.000000), (0.000000, 0.515388, 0.000000), (0.000000, -0.515388, 0.000000), (0.515388, 0.000000, -0.012446) and (-0.515388, 0.000000,-0.012446).

The equation (3) is the eliminated equation. $x_1$ is the reduced variable. We can get the following variable reduction scheme:

$$x_1 = \pm\sqrt{0.265625 - x_2^2} \tag{57}$$

(31) E31:

$$\begin{cases} x_1^2 - x_2 - 2 = 0 \quad (1) \\ x_1 + \sin(\frac{\pi}{2}x_2) = 0 \quad (2) \end{cases} \tag{58}$$

where $x_1 \in [0,1],\ x_2 \in [-10,0]$. It has two roots: $(0,-2)$ and $(0.707660,-1.5)$.

The equation (1) is the eliminated equation. $x_2$ is the reduced variable. We can get the following variable reduction scheme:

$$x_2 = x_1^2 - 2 \tag{59}$$

(32) E32:

$$\begin{cases} x_1^2 + x_2^2 + x_1 + x_2 - 8 = 0 \quad (1) \\ x_1|x_2| + x_1 + |x_2| - 5 = 0 \quad (2) \end{cases} \tag{60}$$

where $x_1 \in [0,2.5],\ x_2 \in [-4,6]$. It has four roots: (0.404634, -3.271577), (2.403604, -0.762837), (1, 2) and (2, 1).

The equation (2) is the eliminated equation. $x_1$ is the reduced variable. We can get the following variable reduction scheme:

$$x_1 = \frac{5 - |x_2|}{|x_2| + 1} \tag{61}$$

(33) E33:

$$\begin{cases} x_1^2 - |x_2| + 1 + \frac{1}{9}|x_1 - 1| = 0 \quad (1) \\ x_2^2 + 5x_1^2 - 7 + \frac{1}{9}|x_2| = 0 \quad (2) \end{cases} \tag{62}$$

where $x_1 \in [-1,1],\ x_2 \in [-10,10]$. It has four roots: (-0.814326, -1.864719), (0.861828, -1.758100), (-0.814326, 1.864719) and (0.861828, 1.758100).

The equation (1) is the eliminated equation. $x_2$ is the reduced variable. We can get the following variable reduction scheme:

$$x_2 = \pm(x_1^2 + 1 + \frac{1}{9}|x_1 - 1|) \tag{63}$$

(34) E34:

$$\begin{cases} 0.5\sin(x_1x_2) - \dfrac{0.25}{\pi}x_2 - 0.5x_1 = 0 & (1) \\ (1 - \dfrac{0.25}{\pi})(e^{2x_1} - e) + \dfrac{e}{\pi}x_2 - 2ex_1 = 0 & (2) \end{cases} \tag{64}$$

where $x_1 \in [0.25, 1]$, $x_2 \in [1.5, 2\pi]$. It has two roots: $(0.299465, 2.836948)$ and $(0.499966, 3.141589)$.

The equation (2) is the eliminated equation. $x_2$ is the reduced variable. We can get the following variable reduction scheme:

$$x_2 = 2\pi x_1 - (0.25 - \pi)(e^{2x_1 - 1} - 1) \tag{65}$$

(35) E35:

$$\begin{cases} x_1^{x_2} + x_2^{x_1} - 5x_1x_2x_3 - 85 = 0 & (1) \\ x_1^3 - x_2^{x_3} - x_3^{x_2} - 60 = 0 & (2) \\ x_1^{x_3} + x_3^{x_1} - x_2 - 2 = 0 & (3) \end{cases} \tag{66}$$

where $x_1 \in [3, 5]$, $x_2 \in [2, 4]$, $x_3 \in [0.5, 2]$. It has one root: $(4, 3, 1)$.

The equation (3) is the eliminated equation. $x_2$ is the reduced variable. We can get the following variable reduction scheme:

$$x_2 = x_1^{x_3} + x_3^{x_1} - 2 \tag{67}$$

(36) E36:

$$\begin{cases} x_1^3 - 3x_1x_2^2 - 1 = 0 & (1) \\ 3x_1^2x_2 - x_2^3 + 1 = 0 & (2) \end{cases} \tag{68}$$

where $x_1 \in [-1, -0.1]$, $x_2 \in [-2, 2]$. It has two roots: (-0.793701,- 0.793701) and (-0.290515,1.084215).

The equation (1) is the eliminated equation. $x_2$ is the reduced variable. We can get the following variable reduction scheme:

$$x_2 = \pm\sqrt{\frac{x_1^3 - 1}{3x_1}} \tag{69}$$

(37) E37:

$$\begin{cases} 0.1x_1 + \cos(2x_2) + 0.09240 = 0 & (1) \\ \sin(3x_3) + \sin(\dfrac{10\sin x_1}{3}) + \ln(2x_2) - 2.52x_3 + 0.08805 = 0 & (2) \\ 2(x_1 - 0.75)^2 + \sin(16\pi x_2 - \dfrac{\pi}{2}) - 3.26815 = 0 & (3) \end{cases} \tag{70}$$

where $x_1 \in [1, 2.5]$, $x_2 \in [0.2, 2]$, $x_3 \in [0.1, 3]$. It has one roots: (1.852100,0.926050,0.617370).

The equation (1) is the eliminated equation. $x_1$ is the reduced variable. We can get the following variable reduction scheme:

$$x_1 = -10\cos(2x_2) - 0.924 \tag{71}$$

(38) E38:

$$\begin{cases} 4x_1^3 - 3x_1 - x_2 = 0 & (1) \\ x_1^2 - x_2 = 0 & (2) \end{cases} \tag{72}$$

where $x_1 \in [-5, 1.5]$, $x_2 \in [0, 5]$. It has three roots: $(-0.75, 0.5625)$, $(0, 0)$ and $(1, 1)$.

The equation (2) is the eliminated equation. $x_2$ is the reduced variable. We can get the following variable reduction scheme:

$$x_2 = x_1^2 \tag{73}$$

(39) E39:

$$\begin{cases} x_1^3 - 3x_1x_2^2 + a_1(2x_1^2 + x_1x_2) + b_2x_2^2 + c_1x_1 + a_2x_2 = 0 & (1) \\ 3x_1^2x_2 - x_2^3 - a_1(4x_1x_2 - x_2^2) + b_2x_1^2 + c_2 = 0 & (2) \end{cases} \tag{74}$$

where $x_1 \in [0, 2]$, $x_2 \in [10, 30]$ and $a_1 = 25$, $b_1 = 1$, $c_1 = 2$, $a_2 = 3$, $b_2 = 4$, $c_2 = 5$. It has two roots: (1.6359718,13.8476653) and (0.6277425,22.2444123).

The equation (2) is the eliminated equation. $x_1$ is the reduced variable. We can get the following variable reduction scheme:

$$x_1 = \frac{50x_2 \pm \sqrt{3x_2^4 - 71x_2^3 + 2400x_2^2 - 15x_2 - 20}}{3x_2 + 4} \tag{75}$$

(40) E40:

$$\begin{cases} x_1^2 - x_1 - x_2^2 - x_2 + x_3^2 = 0 & (1) \\ \sin(x_2 - e^{x_1}) = 0 & (2) \\ x_3 - \ln(|x_2|) = 0 & (3) \end{cases} \tag{76}$$

where $x_1 \in [0, 2]$, $x_2 \in [-10, 10]$, $x_3 \in [-1, 1]$. It has five roots: (0.825297, -0.859034, -0.151946), (1.299490, 0.525835, -0.642769), (1.533662,

-1.648068, 0.499604), (1.981360, -2.172180, 0.775731) and (1.983283, 0.983378, -0.016762)

The equation (3) is regarded as the eliminated equation. $x_3$ is the reduced variable. We can get the following variable reduction scheme:

$$x_3 = \ln(|x_2|) \tag{77}$$

(41) E41:

$$\begin{cases} x_1^4 + 4x_2^4 - 6.0 = 0 & (1) \\ x_1^2 x_2 - 0.6787 = 0 & (2) \end{cases} \tag{78}$$

where $x_1 \in [-2, 2],\ x_2 \in [0, 1.1]$. It has four roots: (-1.563533, 0.277628), (0.789706, 1.088295), (1.563533, 0.277628) and (-0.789706, 1.088295).

The equation (2) is the eliminated equation. $x_1$ is the reduced variable. We can get the following variable reduction scheme:

$$x_1 = \pm\sqrt{\frac{0.6787}{x_2}} \tag{79}$$

(42) E42:

$$\begin{cases} \frac{0.25}{\pi} x_2 + 0.5x_1 - 0.5\sin(x_1 x_2) = 0 & (1) \\ \frac{e}{\pi} x_2 - 2ex_1 + (1 - \frac{0.25}{\pi})(e^{2x_1} - e) = 0 & (2) \end{cases} \tag{80}$$

where $x_1 \in [0.25, 1],\ x_2 \in [1.5, 2\pi]$. It has two roots: $(0.5, \pi)$ and $(0.2995, 2.8369)$.

The equation (2) is the eliminated equation. $x_2$ is the reduced variable. We can get the following variable reduction scheme:

$$x_2 = 2\pi x_1 - (\pi - 0.25)(e^{2x_1 - 1} - 1) \tag{81}$$

(43) E43-Chemical equilibrium application:

$$\begin{cases} x_1 x_2 + x_1 - 3x_5 = 0 & (1) \\ 2x_1 x_2 + x_1 + x_2 x_3^2 + R_8 x_2 - R x_5 + \\ 2R_{10} x_2^2 + R_7 x_2 x_3 + R_9 x_2 x_4 = 0 & (2) \\ 2x_2 x_3^2 + 2R_5 x_3^2 - 8x_5 + R_6 x_3 + R_7 x_2 x_3 = 0 & (3) \\ R_9 x_2 x_4 + 2x_4^2 - 4R x_5 = 0 & (4) \\ x_1(x_2 + 1) + R_{10} x_2^2 + x_2 x_3^2 + R_8 x_2 + \\ R_5 x_3^2 + x_4^2 - 1 + R_6 x_3 + R_7 x_2 x_3 + R_9 x_2 x_4 = 0 & (5) \end{cases} \tag{82}$$

where $x_1, x_5 \in [0, 1],\ x_2 \in [0, 60],\ x_3, x_4 \in [-1, 1]$ and $R = 10.0,\ R_5 = 0.193,\ R_6 = \frac{0.002597}{\sqrt{40}},\ R_7 = \frac{0.003448}{\sqrt{40}},\ R_8 = \frac{0.00001799}{40},$ $R_9 = \frac{0.0002155}{\sqrt{40}},\ R_{10} = \frac{0.00003846}{40}$. It has infinitely many optimal solutions.

The equation (1) and (4) are the eliminated equations. $x_1$ and $x_5$ are the reduced variables. We can get the following variable reduction scheme:

$$\begin{aligned} x_1 &= \frac{3(2x_4^2 + \mathrm{R}_9 x_2 x_4)}{4\mathrm{R}(x_2 + 1)} \\ x_5 &= \frac{x_4^2}{2\mathrm{R}} + \frac{\mathrm{R}_9 x_2 x_4}{4\mathrm{R}} \end{aligned} \tag{83}$$

(44) E44- Neurophysiology application model:

$$\begin{cases} x_1^2 + x_3^2 = 1 & (1) \\ x_2^2 + x_4^2 = 1 & (2) \\ x_5 x_3^3 + x_6 x_4^3 - c_1 = 0 & (3) \\ x_5 x_1^3 + x_6 x_2^3 - c_2 = 0 & (4) \\ x_5 x_1 x_3^2 + x_6 x_4^2 x_2 - c_3 = 0 & (5) \\ x_5 x_3 x_1^2 + x_6 x_2^2 x_4 - c_4 = 0 & (6) \end{cases} \tag{84}$$

where $x_i \in [-10, 10],\ i = 1, 2, \cdots, D$ and $D = 6$, $c_j = 0,\ j = 1, 2, \cdots, 4$. It has infinitely many optimal solutions.

The equation (1), (2) and (3) are the eliminated equations. $x_1$, $x_2$ and $x_6$ are the reduced variables. We can get the following variable reduction scheme:

$$\begin{aligned} x_1 &= \pm\sqrt{1 - x_3^2} \\ x_2 &= \pm\sqrt{1 - x_4^2} \\ x_6 &= -x_5 x_3^3 / x_4^3 \end{aligned} \tag{85}$$

(45) E45- Combustion theory application model:

$$\begin{cases} x_2 + 2x_6 + x_9 + 2x_{10} - 10^{-5} = 0 & (1) \\ x_3 + x_8 - 3\times 10^{-5} = 0 & (2) \\ x_1 + x_3 + 2x_5 + 2x_8 + x_9 + x_{10} - 5\times 10^{-5} = 0 & (3) \\ x_4 + x_7 - 10^{-5} = 0 & (4) \\ 0.5140437\times 10^{-7} x_5 - x_1^2 = 0 & (5) \\ 0.1006932\times 10^{-6} x_6 - 2x_2^2 = 0 & (6) \\ 0.7816278\times 10^{-15} x_7 - x_4^2 = 0 & (7) \\ 0.1496236\times 10^{-6} x_8 - x_1 x_3 = 0 & (8) \\ 0.6194411\times 10^{-7} x_9 - x_1 x_2 = 0 & (9) \\ 0.2089296\times 10^{-14} x_{10} - x_1 x_2^2 = 0 & (10) \end{cases} \tag{86}$$

where $x_i \in [-10,10]$, $i = 1,2,\cdots,D$ and $D = 10$. It has infinitely many optimal solutions.

The equation (1), (2), (3) and (4) are the eliminated equations. $x_1$, $x_2$, $x_3$ and $x_4$ are the reduced variables. We can get the following variable reduction scheme:

$$\begin{aligned} x_1 &= \frac{1}{50000} - x_8 - x_9 - x_{10} - 2x_5 \\ x_2 &= \frac{1}{100000} - x_9 - 2x_{10} - 2x_6 \\ x_3 &= \frac{3}{100000} - x_8 \\ x_4 &= \frac{1}{100000} - 2x_7 \end{aligned} \tag{87}$$

(46) E46- Economics modeling system:

$$\begin{cases} (x_k + \sum_{i=1}^{D-k-1} x_i x_{i+k}) x_D - c_k = 0 \quad 1 \le k \le D-1 & (1) \\ \sum_{l=1}^{D-1} x_l + 1 = 0 & (2) \end{cases} \tag{88}$$

where $x_i \in [-10,10]$, $i = 1,2,\cdots,D$ and $D = 5$. It has infinitely many optimal solutions.

The equation (2) is the eliminated equation. $x_1$ is the reduced variable. We can get the following variable reduction scheme:

$$x_1 = 1 - \sum_{j=2}^{D-1} x_j \tag{89}$$

The root rate and success rate of the eleven compared methods on test problems E1-E42 (except E5, E12 and E25) are shown in Table S-2 and S-3.

**Table S-2** Root rate of the eleven compared methods on 39 test problems.

| Test problem | VR-DR-JADE | DR-JADE | VR-MONES | MONES | A-WeB | NCDE | NSDE | I-HS | GA-SQP | PSO-NM | NCSA |
|---|---|---|---|---|---|---|---|---|---|---|---|
| E1 | **1.0000** | **1.0000** | **1.0000** | **1.0000** | 0.7250 | **1.0000** | **1.0000** | **1.0000** | 0.7667 | **1.0000** | 0.9833 |
| E2 | **1.0000** | **1.0000** | **1.0000** | 0.9778 | 0.8800 | **1.0000** | 0.9778 | 0.9667 | 0.7000 | 0.9556 | 0.8444 |
| E3 | **1.0000** | 0.8667 | 0.0000 | 0.0000 | 0.5450 | 0.9897 | 0.9256 | 0.7000 | 0.2000 | 0.4000 | 0.3000 |
| E4 | **1.0000** | **1.0000** | **1.0000** | **1.0000** | **1.0000** | **1.0000** | **1.0000** | **1.0000** | 0.6667 | **1.0000** | **1.0000** |
| E6 | **1.0000** | **1.0000** | **1.0000** | **1.0000** | 0.8300 | **1.0000** | **1.0000** | 0.9000 | 0.9000 | 0.8333 | 0.0500 |
| E7 | **1.0000** | **1.0000** | **1.0000** | **1.0000** | **1.0000** | **1.0000** | **1.0000** | **1.0000** | 0.7667 | 0.9111 | 0.9667 |
| E8 | **1.0000** | **1.0000** | **1.0000** | **1.0000** | **1.0000** | **1.0000** | **1.0000** | **1.0000** | 0.8000 | **1.0000** | 0.9667 |
| E9 | 0.0000 | 0.0000 | **1.0000** | **1.0000** | 0.6200 | 0.9833 | **1.0000** | 0.0000 | 0.0000 | 0.0000 | 0.5667 |
| E10 | **1.0000** | 0.9970 | **1.0000** | 0.9879 | **1.0000** | 0.9848 | 0.9485 | 0.6970 | 0.2424 | 0.8182 | 0.6061 |
| E11 | **1.0000** | 0.9378 | **1.0000** | 0.4889 | 0.9573 | 0.9778 | 0.9644 | 0.4844 | 0.2000 | 0.6844 | 0.4444 |
| E13 | **1.0000** | **1.000** | **1.0000** | **1.0000** | **1.0000** | **1.0000** | 0.9333 | 0.2667 | **1.0000** | 0.8667 | **1.0000** |
| E14 | **1.0000** | 0.9667 | 0.6542 | 0.1250 | 0.9400 | 0.8708 | 0.8833 | 0.8208 | 0.1875 | 0.8750 | 0.5375 |
| E15 | **1.0000** | **1.0000** | **1.0000** | 0.0333 | 0.4200 | 0.0667 | 0.1333 | 0.0333 | 0.6000 | **1.0000** | **1.0000** |
| E16 | 0.8571 | **1.0000** | 0.8667 | 0.4476 | 0.8371 | 0.919 | 0.9238 | 0.6762 | 0.4381 | 0.8952 | 0.5333 |
| E17 | **1.0000** | **1.0000** | 0.5667 | 0.0778 | 0.8933 | 0.0000 | 0.0111 | 0.8778 | 0.6333 | 0.6444 | 0.5444 |
| E18 | **1.0000** | **1.0000** | **1.0000** | **1.0000** | **1.0000** | **1.0000** | **1.0000** | **1.0000** | 0.9333 | 0.7333 | **1.0000** |
| E19 | **1.0000** | 0.8600 | **1.0000** | 0.4300 | 0.8880 | 0.9933 | 0.9533 | 0.7933 | 0.1133 | 0.5933 | 0.5200 |
| E20 | **1.0000** | **1.0000** | 0.7778 | 0.3111 | 0.9733 | 0.9185 | 0.9333 | 0.7667 | 0.2259 | 0.3926 | 0.5222 |
| E22 | 0.8729 | 0.8375 | 0.2146 | 0.0813 | 0.6688 | 0.9917 | 0.9896 | 0.8063 | 0.1375 | 0.0667 | 0.2125 |
| E23 | **1.0000** | **1.0000** | **1.0000** | 0.6556 | 0.9433 | 0.9944 | **1.0000** | 0.8944 | 0.4889 | 0.8333 | 0.7722 |
| E24 | **1.0000** | 0.0000 | **1.0000** | 0.0000 | 0.6200 | 0.0000 | 0.0000 | 0.0000 | 0.0000 | 0.0000 | 0.0333 |
| E25 | **1.0000** | **1.0000** | 0.7095 | 0.5952 | 0.9514 | 0.9762 | 0.9952 | 0.6857 | 0.5286 | 0.8952 | 0.6762 |
| E26 | **1.0000** | **1.0000** | **1.0000** | 0.5250 | 0.9950 | **1.0000** | **1.0000** | **1.0000** | 0.5000 | 0.6833 | 0.9000 |
| E27 | **1.0000** | **1.0000** | **1.0000** | 0.5000 | **1.0000** | **1.0000** | 0.9944 | 0.9833 | 0.4389 | 0.7778 | 0.7222 |
| E28 | **1.0000** | 0.9208 | 0.9875 | 0.7000 | 0.8550 | **1.0000** | **1.0000** | 0.4750 | 0.4000 | 0.7500 | 0.5500 |
| E29 | **1.0000** | **1.0000** | 0.9667 | 0.5000 | **1.0000** | **1.0000** | 0.9833 | 0.9833 | 0.6167 | 0.8000 | 0.9000 |
| E30 | 0.8833 | 0.9306 | 0.3611 | 0.6333 | 0.0933 | 0.9750 | 0.9389 | 0.9222 | 0.2833 | 0.4778 | 0.4278 |
| E31 | **1.0000** | **1.0000** | **1.0000** | **1.0000** | **1.0000** | 0.7833 | 0.9167 | 0.9833 | 0.6333 | **1.0000** | 0.9167 |
| E32 | **1.0000** | **1.0000** | **1.0000** | 0.9250 | **1.0000** | 0.9167 | 0.9917 | **1.0000** | 0.4667 | 0.8833 | 0.8833 |
| E33 | **1.0000** | **1.0000** | **1.0000** | 0.5000 | **1.0000** | 0.4500 | 0.9250 | **1.0000** | 0.4583 | 0.9000 | 0.8583 |
| E34 | **1.0000** | 0.5000 | **1.0000** | 0.9500 | **1.0000** | 0.0000 | 0.0000 | 0.9167 | 0.5500 | **1.0000** | 0.4333 |
| E35 | **1.0000** | **1.0000** | 0.0667 | **1.0000** | **1.0000** | 0.0000 | 0.0000 | **1.0000** | 0.1333 | **1.0000** | **1.0000** |

| | | | | | | | | | | | |
|---|---|---|---|---|---|---|---|---|---|---|---|
| E36 | **1.0000** | **1.0000** | **1.0000** | **1.0000** | **1.0000** | **1.0000** | **1.0000** | **1.0000** | 0.65 | **1.0000** | 0.9833 |
| E37 | **1.0000** | **1.0000** | **1.0000** | 0.5000 | 0.8800 | 0.3667 | 0.8667 | **1.0000** | 0.1667 | 0.8000 | **1.0000** |
| E38 | **1.0000** | **1.0000** | **1.0000** | **1.0000** | **1.0000** | 0.7889 | 0.9889 | 0.9556 | 0.7222 | 0.9778 | 0.8556 |
| E39 | **1.0000** | **1.0000** | **1.0000** | 0.5000 | 0.9400 | 0.3000 | 0.5000 | 0.9333 | 0.0000 | **1.0000** | 0.7500 |
| E40 | 0.9867 | 0.9467 | 0.8467 | 0.5333 | 0.9320 | 0.8067 | 0.8600 | 0.9933 | 0.2200 | 0.8400 | 0.7200 |
| E41 | **1.0000** | **1.0000** | 0.5000 | **1.0000** | **1.0000** | 0.9917 | **1.0000** | 0.9833 | 0.5250 | 0.9000 | 0.8167 |
| E42 | **1.0000** | **1.0000** | **1.0000** | **1.0000** | 0.9900 | 0.9833 | **1.0000** | **1.0000** | 0.5667 | **1.0000** | 0.9833 |
| Avg. | **0.9641** | 0.9170 | 0.8594 | 0.6661 | 0.8815 | 0.7956 | 0.8343 | 0.8077 | 0.4579 | 0.7741 | 0.7123 |

**Table S-3** Success rate of the eleven compared methods on 39 test problems.

| Test problem | VR-DR-JADE | DR-JADE | VR-MONES | MONES | A-WeB | NCDE | NSDE | I-HS | GA-SQP | PSO-NM | NCSA |
|---|---|---|---|---|---|---|---|---|---|---|---|
| E1 | **1.0000** | **1.0000** | **1.0000** | **1.0000** | 0.5300 | **1.0000** | **1.0000** | **1.0000** | 0.5333 | **1.0000** | 0.9667 |
| E2 | **1.0000** | **1.0000** | **1.0000** | 0.9333 | 0.6800 | 1.0000 | 0.9333 | 0.9000 | 0.3667 | 0.8667 | 0.5667 |
| E3 | **1.0000** | 0.7333 | 0.0000 | 0.0000 | 0.2000 | 0.8667 | 0.3667 | 0.5300 | 0.0000 | 0.0667 | 0.0000 |
| E4 | **1.0000** | **1.0000** | **1.0000** | **1.0000** | **1.0000** | **1.0000** | **1.0000** | **1.0000** | 0.3333 | **1.0000** | **1.0000** |
| E6 | **1.0000** | **1.0000** | **1.0000** | **1.0000** | 0.6500 | **1.0000** | **1.0000** | 0.8300 | 0.8000 | 0.6667 | 0.0000 |
| E7 | **1.0000** | **1.0000** | **1.0000** | **1.0000** | **1.0000** | **1.0000** | **1.0000** | **1.0000** | 0.4000 | 0.7333 | 0.9000 |
| E8 | **1.0000** | **1.0000** | **1.0000** | **1.0000** | **1.0000** | **1.0000** | **1.0000** | **1.0000** | 0.6000 | **1.0000** | 0.9333 |
| E9 | 0.0000 | 0.0000 | **1.0000** | **1.0000** | 0.3600 | 0.9667 | 1.0000 | 0.0000 | 0.0000 | 0.0000 | 0.1333 |
| E10 | **1.0000** | 0.9667 | **1.0000** | 0.9000 | **1.0000** | 0.8333 | 0.5667 | 0.0000 | 0.0000 | 0.0000 | 0.0000 |
| E11 | **1.0000** | 0.2667 | **1.0000** | 0.0000 | 0.5800 | 0.8000 | 0.6333 | 0.0000 | 0.0000 | 0.0000 | 0.0000 |
| E13 | **1.0000** | **1.0000** | **1.0000** | **1.0000** | **1.0000** | **1.0000** | 0.9333 | 0.2667 | **1.0000** | 0.8667 | **1.0000** |
| E14 | **1.0000** | 0.7333 | 0.0000 | 0.0000 | 0.6000 | 0.3000 | 0.2667 | 0.1667 | 0.0000 | 0.2667 | 0.0000 |
| E15 | **1.0000** | **1.0000** | **1.0000** | 0.0333 | 0.4200 | 0.0667 | 0.1333 | 0.0333 | 0.6000 | **1.0000** | **1.0000** |
| E16 | 0.0000 | **1.0000** | 0.0667 | 0.0000 | 0.1200 | 0.4333 | 0.5000 | 0.0000 | 0.0000 | 0.3333 | 0.0000 |
| E17 | **1.0000** | **1.0000** | 0.0667 | 0.0000 | 0.6800 | 0.0000 | 0.0000 | 0.6667 | 0.0667 | 0.0667 | 0.1000 |
| E18 | **1.0000** | **1.0000** | **1.0000** | **1.0000** | **1.0000** | **1.0000** | **1.0000** | **1.0000** | 0.9333 | 0.7333 | **1.0000** |
| E19 | **1.0000** | 0.0333 | **1.0000** | 0.0000 | 0.2800 | 0.9333 | 0.8000 | 0.0000 | 0.0000 | 0.0000 | 0.0000 |
| E20 | **1.0000** | **1.0000** | 0.0000 | 0.0000 | 0.7600 | 0.4000 | 0.4667 | 0.0000 | 0.0000 | 0.0000 | 0.0000 |
| E22 | 0.0667 | 0.0333 | 0.0000 | 0.0000 | 0.0000 | 0.8667 | 0.9000 | 0.0000 | 0.0000 | 0.0000 | 0.0000 |
| E23 | **1.0000** | **1.0000** | **1.0000** | 0.0000 | 0.6600 | 0.9667 | **1.0000** | 0.4667 | 0.0000 | 0.2000 | 0.0667 |
| E24 | **1.0000** | 0.0000 | **1.0000** | 0.0000 | 0.2400 | 0.0000 | 0.0000 | 0.0000 | 0.0000 | 0.0000 | 0.0000 |
| E25 | **1.0000** | **1.0000** | 0.0000 | 0.0000 | 0.7000 | 0.8333 | 0.9667 | 0.0333 | 0.0000 | 0.3333 | 0.0000 |
| E26 | **1.0000** | **1.0000** | **1.0000** | 0.0000 | 0.9800 | **1.0000** | **1.0000** | **1.0000** | 0.0333 | 0.2000 | 0.6333 |
| E27 | **1.0000** | **1.0000** | **1.0000** | 0.0000 | **1.0000** | **1.0000** | 0.9667 | 0.9000 | 0.0000 | 0.2667 | 0.0667 |
| E28 | **1.0000** | 0.5000 | 0.9000 | 0.0000 | 0.1400 | **1.0000** | **1.0000** | 0.0000 | 0.0000 | 0.1333 | 0.0000 |
| E29 | **1.0000** | **1.0000** | 0.9333 | 0.0000 | **1.0000** | **1.0000** | 0.9667 | 0.9667 | 0.2333 | 0.6000 | 0.8000 |
| E30 | 0.3333 | 0.2667 | 0.0000 | 0.0000 | 0.0000 | 0.7667 | 0.4667 | 0.2667 | 0.0000 | 0.0000 | 0.0000 |
| E31 | **1.0000** | **1.0000** | **1.0000** | **1.0000** | **1.0000** | 0.5667 | 0.8333 | 0.9667 | 0.3667 | **1.0000** | 0.8333 |
| E32 | **1.0000** | **1.0000** | **1.0000** | 0.7000 | **1.0000** | 0.6667 | 0.9667 | **1.0000** | 0.0000 | 0.5333 | 0.5667 |
| E33 | **1.0000** | **1.0000** | **1.0000** | 0.0000 | **1.0000** | 0.0333 | 0.7667 | **1.0000** | 0.0000 | 0.6000 | 0.5000 |
| E34 | **1.0000** | 0.0000 | **1.0000** | 0.9000 | **1.0000** | 0.0000 | 0.0000 | 0.8333 | 0.3667 | **1.0000** | 0.0000 |
| E35 | **1.0000** | **1.0000** | 0.0667 | **1.0000** | **1.0000** | 0.0000 | 0.0000 | **1.0000** | 0.1333 | **1.0000** | **1.0000** |
| E36 | **1.0000** | **1.0000** | **1.0000** | **1.0000** | **1.0000** | **1.0000** | **1.0000** | **1.0000** | 0.4333 | **1.0000** | 0.9667 |
| E37 | **1.0000** | **1.0000** | **1.0000** | 0.5000 | 0.8800 | 0.3667 | 0.8667 | **1.0000** | 0.1667 | 0.8000 | **1.0000** |
| E38 | **1.0000** | **1.0000** | **1.0000** | **1.0000** | **1.0000** | 0.4333 | 0.9667 | 0.8667 | 0.2333 | 0.9333 | 0.5667 |
| E39 | **1.0000** | **1.0000** | **1.0000** | 0.0000 | 0.8800 | 0.0000 | 0.0000 | 0.8667 | 0.0000 | **1.0000** | 0.5000 |
| E40 | 0.9333 | 0.7333 | 0.5333 | 0.0000 | 0.6600 | 0.3333 | 0.5000 | 0.9667 | 0.0000 | 0.4000 | 0.1667 |
| E41 | **1.0000** | **1.0000** | 0.0000 | **1.0000** | **1.0000** | 0.9667 | **1.0000** | 0.9333 | 0.0333 | 0.6667 | 0.3333 |
| E42 | **1.0000** | **1.0000** | **1.0000** | **1.0000** | 0.9900 | 0.9666 | **1.0000** | **1.0000** | 0.4000 | **1.0000** | 0.9667 |
| Avg. | **0.9060** | 0.8017 | 0.7325 | 0.4607 | 0.7177 | 0.6761 | 0.7120 | 0.6015 | 0.2060 | 0.5197 | 0.4248 |
